# Supplementary material for: Towards Autonomous Micromobility through Scalable Urban Simulation
Source: arXiv:2505.00690 source file (2025-05-01)
Supplement: Supplementary file 1 [file 6_evaluation.tex]

\section{Evaluation of Critical Questions}
\label{sec:evaluations}
